# Supplementary material for: Face Beautification: Beyond Makeup Transfer
Source: arXiv:1912.03630 source file (2019-12-11)
Supplement: Supplementary file 1 [file Appendix.tex]

%%
%% If your work has an appendix, this is the place to put it.
%\appendix
%\section{Research Methods}

In contrast, our method directly regress the 3D vertex positions of the mesh using a pre-trained facial recognition network which is then fine-tuned for face reconstruction. Since a person's identity is strongly associated with his shape features \cite{liu2018disentangling}, this allowed us to utilize rich discriminative information to obtain 3D geometries with superior accuracy.

In contrast, our approach encodes mid and higher frequency information in normal and texture maps, thus is much more light-weighted and suitable for production. This has made their method to be robust under difficult conditions, such as when occlusion and out of plane rotations are present. However, their method encodes mid frequency details in the geometry and not the texture, and thus requires a substantial number of vertices to reconstruct high-fidelity geometries.

Similar to our method, they adopted an identity-based loss
